# Supplementary material for: Detecting Hidden Webcams with Delay-Tolerant Similarity of Simultaneous Observation
Source: arXiv:1901.02818 source file (2020-03-27)
Supplement: Supplementary file 1 [file appendices.tex]

\appendices

\section{Tables of Results}
\label{sec:appendixa}

%TODO:  Put the tables here
\begin{table*}[h]
\definecolor{header}{rgb}{0.7,0.7,0.7}
\definecolor{section1}{rgb}{0.74, 0.83, 0.9}
\definecolor{section2}{RGB}{240, 204, 176}
\definecolor{highlight}{rgb}{0.94,0.86,0.51}
\definecolor{bad-highlight}{RGB}{242, 160, 157}

\footnotesize
\centering
%\begin{minipage}{0.4\paperwidth}
 \begin{tabular}{|c|c|c|c|}\hline
   \multicolumn{2}{|c|}{\bfseries\cellcolor{header}Testing samples} & \bfseries\cellcolor{header}Average & \bfseries\cellcolor{header}Standard deviation \\\hline\hline
   
  \multicolumn{4}{|l|}{\cellcolor{section1}\bfseries Wi-Fi camera} \\\hline
  \multicolumn{2}{|c|}{\cellcolor{highlight}No motion}       &\cellcolor{highlight}  $0.3037$ &\cellcolor{highlight}  $0.1718$ \\\hline
  \multirow{3}{*}{Motion} &   0 degree  &  $0.6028 $ & $0.1725$ \\\cline{2-4}
                          &  90 degrees &  $0.3865 $ & $0.3175$ \\\cline{2-4}
                          & 180 degrees &  $0.4027 $ & $0.2109$ \\\hline
  \multicolumn{2}{|c|}{Campus}          &  $0.3040 $ & $0.2726$ \\\hline
  
  \multicolumn{4}{|l|}{\cellcolor{section2}\bfseries Other non-spying camera traffics}\\\hline
  \multicolumn{2}{|c|}{Amazon TV}         & $-0.0101$           & $0.0975$ \\\hline
  \multicolumn{2}{|c|}{Switch gaming}     & $\phantom{-}0.0649$ & $0.0877$ \\\hline
  \multicolumn{2}{|c|}{Normal browsing}   & $-0.0256$           & $0.1523$ \\\hline
  \multicolumn{2}{|c|}{Skype}             & $\phantom{-}0.0020$ & $0.1436$ \\\hline
  \multicolumn{2}{|c|}{Video downloading} & $-0.0022$           & $0.0979$ \\\hline
  \multicolumn{2}{|c|}{YouTube}           & $-0.0070$           & $0.1106$ \\\hline
  \multicolumn{2}{|c|}{YouTube TV}        & $\phantom{-}0.0272$ & $0.0880$ \\\hline
  		\noalign{\vskip 1mm}   
 \end{tabular}
%  \end{minipage}
 % \begin{minipage}{0.6\paperwidth}
 
%   \begin{tabular}{|c|c|c|c|}\hline
%   \multicolumn{2}{|c|}{\bfseries\cellcolor{header}Testing samples} & \bfseries\cellcolor{header}Average & \bfseries\cellcolor{header}Standard deviation \\\hline\hline

%   \multicolumn{4}{|l|}{\cellcolor{section1}\bfseries Wi-Fi camera} \\\hline
%   \multicolumn{2}{|c|}{No motion}       & $0.011453722$ & $0.005228987$ \\\hline
%   \multirow{3}{*}{Motion} &   0 degree  & $0.005479047$ & $0.003783815$ \\\cline{2-4}
%                           &  90 degrees & $0.009357307$ & $0.014222304$ \\\cline{2-4}
%                           & 180 degrees & $0.007548263$ & $0.006156813$ \\\hline
%   \multicolumn{2}{|c|}{Campus}          & $0.028721493$ & $0.028825679$ \\\hline
  
%   \multicolumn{4}{|l|}{\cellcolor{section2}\bfseries Other non-spying camera traffics}\\\hline
%   \multicolumn{2}{|c|}{Amazon TV}         & $0.069038229$ & $0.026416606$ \\\hline
%   \multicolumn{2}{|c|}{Switch gaming}     & $0.037086219$ & $0.015433377$ \\\hline
%   \multicolumn{2}{|c|}{Normal browsing}   & $8.394858985$ & $4.355179579$ \\\hline
%   \multicolumn{2}{|c|}{Skype}             & $0.038609769$ & $0.099741421$ \\\hline
%   \multicolumn{2}{|c|}{Video downloading} & $0.063745689$ & $0.055284152$ \\\hline
%   \multicolumn{2}{|c|}{YouTube}           & $1.471183735$ & $1.268920535$ \\\hline
%   \multicolumn{2}{|c|}{YouTube TV}        & $0.047435962$ & $0.015764356$ \\\hline
%  \end{tabular}
%  \end{minipage}

 \caption{Result of the CC for Wi-Fi camera-based detection model.}
 \label{wifi-cc}
 
\end{table*}

\begin{table*}[h]
\definecolor{header}{rgb}{0.7,0.7,0.7}
\definecolor{header2}{rgb}{0.8,0.8,0.8}
\definecolor{section1}{rgb}{0.74, 0.83, 0.9}
\definecolor{section2}{RGB}{240, 204, 176}
\definecolor{highlight}{rgb}{0.94,0.86,0.51}
\definecolor{bad-highlight}{RGB}{242, 160, 157}

\centering
\footnotesize
\begin{tabular}{|c|c|c|>{\centering\arraybackslash}p{1.8cm}|c|>{\centering\arraybackslash}p{1.8cm}|}\hline
  \multicolumn{2}{|c|}{\cellcolor{header}} & \multicolumn{2}{c|}{\bfseries\cellcolor{header} KLD} & \multicolumn{2}{c|}{\bfseries\cellcolor{header} JSD} \\\hhline{|>{\arrayrulecolor{header}}--%
  >{\arrayrulecolor{black}}|----}
  \multicolumn{2}{|c|}{\cellcolor{header}\bfseries Testing samples}& \bfseries\cellcolor{header2}\multirow{2}{*}{Average} & \bfseries\cellcolor{header2}Standard deviation & \bfseries\cellcolor{header2}\multirow{2}{*}{Average} & \bfseries\cellcolor{header2}Standard deviation \\\hline\hline
  
  \multicolumn{6}{|l|}{\cellcolor{section1}\bfseries Wi-Fi camera} \\\hline
  \multicolumn{2}{|c|}{\cellcolor{highlight}No motion}       &\cellcolor{highlight} $0.0114$ &\cellcolor{highlight} $0.0052$ &\cellcolor{highlight} $0.0028$ &\cellcolor{highlight} $0.0012$ \\\hline
  \multirow{3}{*}{Motion} &   0 degree  & $0.0054$ & $0.0037$ & $0.0013$ & $0.0009$ \\\cline{2-6}
                          &  90 degrees & $0.0093$ & $0.0142$ & $0.0022$ & $0.0024$ \\\cline{2-6}
                          & 180 degrees & $0.0075$ & $0.0061$ & $0.0018$ & $0.0013$ \\\hline
  \multicolumn{2}{|c|}{Campus}          & $0.0287$ & $0.0288$ &\cellcolor{highlight} $0.0073$ &\cellcolor{highlight} $0.0073$ \\\hline
  
  \multicolumn{6}{|l|}{\cellcolor{section2}\bfseries Other non-spying camera traffics}\\\hline
  \multicolumn{2}{|c|}{Amazon TV}         & $0.0690$ & $0.0264$ & $0.0171$ & $0.0064$\\\hline
  \multicolumn{2}{|c|}{Switch gaming}     & $0.0370$ & $0.0154$ & $0.0086$ & $0.0034$\\\hline
  \multicolumn{2}{|c|}{Normal browsing}   & $8.3948$ & $4.3551$ & $0.3569$ & $0.1180$\\\hline
  \multicolumn{2}{|c|}{Skype}             & $0.0386$ & $0.0997$ & $0.0090$ & $0.0199$\\\hline
  \multicolumn{2}{|c|}{Video downloading} & $0.0637$ & $0.0552$ & $0.0151$ & $0.0121$\\\hline
  \multicolumn{2}{|c|}{YouTube}           & $1.4711$ & $1.2689$ & $0.2916$ & $0.1468$\\\hline
  \multicolumn{2}{|c|}{YouTube TV}        & $0.0474$ & $0.0157$ & $0.0118$ & $0.0038$\\\hline
  		\noalign{\vskip 1mm}   
 \end{tabular}
 
 \caption{Result of the KLD and JSD for Wi-Fi camera-based detection model.}
 \label{wifi-kld-n-jsd}
\end{table*}

\begin{table*}[h]
\definecolor{header}{rgb}{0.7,0.7,0.7}
\definecolor{section1}{rgb}{0.74, 0.83, 0.9}
\definecolor{section2}{RGB}{240, 204, 176}
\definecolor{highlight}{rgb}{0.94,0.86,0.51}
\definecolor{bad-highlight}{RGB}{242, 160, 157}

\footnotesize
\centering
 \begin{tabular}{|c|c|c|c|}\hline
   \multicolumn{2}{|c|}{\bfseries\cellcolor{header}Testing samples} & \bfseries\cellcolor{header}Average & \bfseries\cellcolor{header}Standard deviation \\\hline\hline
   
  \multicolumn{4}{|l|}{\cellcolor{section1}\bfseries Recorded video}   \\\hline
  \multicolumn{2}{|c|}{No motion}      & $11.330$           & $3.757$ \\\hline
  \multirow{3}{*}{720p}  &   0 degree  & $\phantom{0}9.284$ & $2.894$ \\\cline{2-4}
                         &  90 degrees & $\phantom{0}8.951$ & $2.004$ \\\cline{2-4}
                         & 180 degrees & $\phantom{0}8.412$ & $1.806$ \\\hline
  \multirow{3}{*}{1080p} &   0 degree  & $\phantom{0}8.680$ & $2.176$ \\\cline{2-4}
                         &  90 degrees & $\phantom{0}9.611$ & $1.679$ \\\cline{2-4}
                         & 180 degrees & $10.841$           & $6.356$ \\\hline

  \multicolumn{4}{|l|}{\cellcolor{section2}\bfseries Other non-spying camera traffics}\\\hline
  \multicolumn{2}{|c|}{Amazon TV}         & $13.237$ & $4.404$ \\\hline
  \multicolumn{2}{|c|}{Switch gaming}     & $10.573$ & $3.504$ \\\hline
  \multicolumn{2}{|c|}{Normal browsing}   & $22.983$ & $5.867$ \\\hline
  \multicolumn{2}{|c|}{Skype}             & $12.018$ & $6.626$ \\\hline
  \multicolumn{2}{|c|}{Video downloading} & $11.082$ & $3.572$ \\\hline
  \multicolumn{2}{|c|}{YouTube}           & $23.181$ & $6.491$ \\\hline
  \multicolumn{2}{|c|}{YouTube TV}        & $13.564$ & $4.158$ \\\hline
  		\noalign{\vskip 1mm}   
 \end{tabular}
 \caption{Result of the DTW for mobile phone-based detection model.}
 \label{mobile-dtw}
\end{table*}

\begin{table*}[h]
\definecolor{header}{rgb}{0.7,0.7,0.7}
\definecolor{section1}{rgb}{0.74, 0.83, 0.9}
\definecolor{section2}{RGB}{240, 204, 176}
\definecolor{header2}{rgb}{0.8,0.8,0.8}
\definecolor{highlight}{rgb}{0.94,0.86,0.51}
\definecolor{bad-highlight}{RGB}{242, 160, 157}

\centering
\footnotesize

 \begin{tabular}{|c|c|c|>{\centering\arraybackslash}p{1.8cm}|c|>{\centering\arraybackslash}p{1.8cm}|}\hline
  \multicolumn{2}{|c|}{\cellcolor{header}} & \multicolumn{2}{c|}{\bfseries\cellcolor{header} KLD} & \multicolumn{2}{c|}{\bfseries\cellcolor{header} JSD} \\\hhline{|>{\arrayrulecolor{header}}--%
  >{\arrayrulecolor{black}}|----}
  \multicolumn{2}{|c|}{\cellcolor{header}\bfseries Testing samples}& \bfseries\cellcolor{header2}\multirow{2}{*}{Average} & \bfseries\cellcolor{header2}Standard deviation & \bfseries\cellcolor{header2}\multirow{2}{*}{Average} & \bfseries\cellcolor{header2}Standard deviation \\\hline\hline 
  
  \multicolumn{6}{|l|}{\cellcolor{section1}\bfseries Recorded video}   \\\hline
  \multicolumn{2}{|c|}{\cellcolor{highlight}No motion}      &\cellcolor{highlight} $0.01582$ &\cellcolor{highlight} $0.0267$ &\cellcolor{highlight} $0.0033$ &\cellcolor{highlight} $0.0046$ \\\hline
  \multirow{3}{*}{720p}  &   0 degree  & $0.0043$ & $0.0044$ & $0.0010$ & $0.0011$ \\\cline{2-6}
                         &  90 degrees & $0.0030$ & $0.0013$ & $0.0007$ & $0.0003$ \\\cline{2-6}
                         & 180 degrees & $0.0081$ & $0.0111$ & $0.0019$ & $0.0022$ \\\hline
  \multirow{3}{*}{1080p} &   0 degree  & $0.0069$ & $0.0066$ & $0.0017$ & $0.0016$ \\\cline{2-6}
                         &\cellcolor{highlight} 90 degrees &\cellcolor{highlight} $0.0050$ &\cellcolor{highlight} $0.0034$ &\cellcolor{highlight} $0.0012$ &\cellcolor{highlight} $0.0008$ \\\cline{2-6}
                         & 180 degrees & $0.0078$ & $0.0141$ & $0.0017$ & $0.0018$ \\\hline
  
  \multicolumn{6}{|l|}{\cellcolor{section2}\bfseries Other non-spying camera traffics}\\\hline
  \multicolumn{2}{|c|}{Amazon TV}         & $0.0627$ & $0.0247$ & $0.0156$ & $0.0061$ \\\hline
  \multicolumn{2}{|c|}{Switch gaming}     & $0.0335$ & $0.0150$ & $0.0077$ & $0.0033$ \\\hline
  \multicolumn{2}{|c|}{Normal browsing}   & $8.2647$ & $4.2918$ & $0.3545$ & $0.1170$ \\\hline
  \multicolumn{2}{|c|}{Skype}             & $0.0324$ & $0.1007$ & $0.0074$ & $0.0202$ \\\hline
  \multicolumn{2}{|c|}{Video downloading} & $0.0580$ & $0.0552$ & $0.0136$ & $0.0121$ \\\hline
  \multicolumn{2}{|c|}{YouTube}           & $1.4634$ & $1.2637$ & $0.2908$ & $0.1471$ \\\hline
  \multicolumn{2}{|c|}{YouTube TV}        & $0.0429$ & $0.0154$ & $0.0107$ & $0.0037$ \\\hline
  		\noalign{\vskip 1mm}   
 \end{tabular}
 \caption{Result of the KLD and JSD for mobile phone-based detection model.}
 \label{mobile-kld-n-jsd}
\end{table*}
